# Supplementary material for: Irony in Emojis: A Comparative Study of Human and LLM Interpretation
Source: arXiv:2501.11241 source file (2025-01-20)
Supplement: Supplementary file 1 [file appendix.tex]

\appendix

\section{Appendix}
